# Supplementary material for: S$^2$AC: Energy-Based Reinforcement Learning with Stein Soft Actor Critic
Source: arXiv:2405.00987 source file (2024-05-02)
Supplement: Supplementary file 1 [file proof_hmc_likelihood.tex]

\subsection{Proof of Theorem~\ref{thm:hmc_entropy}}
\label{sec:hmc_entropy}

\begin{theorem*}
Under condition: the first order derivative $\nabla_{a^l} Q(s,a^l)$ is Lipschitz continuous along each dimension with a Lipschitz constant $\ll 2/\epsilon^2$, \ie $||\nabla_{a^l}^2 Q(s,a^l)||_{\infty}\ll \epsilon^2$, the closed-form of $\log q^T(a^T)$ of HMC sampler is 
\begin{equation*}\small
\log q^T(a^T) = \log q^0(a^0) - \sum_{l = 0}^{L-1} (\epsilon^2/2) \Tr \big(\nabla_{a^l}^2 Q(s,a^{l})\big) 
\end{equation*}
\end{theorem*}

% \begin{align*}
% \nabla_{a^l} a^{l+1}&= \nabla_{a^l} a^{l} + \epsilon \nabla_{a^l} v^{l+1/2} \\
% &= I + \epsilon \nabla_{a^l} v^{l} + \epsilon(\epsilon/2) \nabla_{a^l}^2 Q(s,a^l)\\ 
% & = I + (\epsilon^2/2) \nabla_{a^l}^2 Q(s,a^l)
% \end{align*}
% Here $\nabla_{a^l} v^{l}=0$ because $v^{l}$ and $a^{l}$ are independent by definition of HMC.

\begin{proof}
%In this proof, we omit the state $s$ in $Q(s,a^{l})$ for simplicity of notation.
Using the first two half steps of updates in Eq.\eqref{eq:hmc_update}, we have
\begin{align*}
&a^{l+1}\\
=& a^{l} + \epsilon v^{l+1/2} \\
=& a^{l} + \epsilon \left(v^l + (\epsilon/2) \nabla_{a^l} Q(s,a^l) \right)
%&= a^{l} + \epsilon v^l + (\epsilon^2/2) \nabla_{a^l} Q(s,a^l)
\end{align*}
Write it in the form of $F(a)=a+\epsilon h(a)$, we have $h(a)=v^l + (\epsilon/2) \nabla_{a^l} Q(s,a^l)$. Therefore, 
\begin{align*}
& \nabla_{a^l}h(a) \\
= & \nabla_{a^l} (v^l + (\epsilon/2)\nabla_{a^l} Q(s,a^l))\\
= & (\epsilon/2)\nabla_{a^l}^2 Q(s,a^l)
\end{align*}
Here $\nabla_{a^l} v^{l}=0$ because $v^{l}$ and $a^{l}$ are independent by definition of HMC. According to Proposition~\ref{prop:hmc_invertibility}, the HMC update function $F(a)$ is invertible. When the first order derivative $\nabla_{a^l} Q(s,a^l)$ is Lipschitz continuous along each dimension with a Lipschitz constant no larger than $ 2/\epsilon^2$, \ie $||\nabla_{a^l}^2 Q(s,a^l)||_{\infty}\ll \epsilon^2$, then it satisfies the condition 
\begin{align*}
\epsilon ||\nabla_{a^l} h(a^l)||_{\infty} = \epsilon ||(\epsilon/2)\nabla_{a^l}^2 Q(s,a^l)||_{\infty} \ll 1 
\end{align*}

Hence Theorem~\ref{thm:generic_entropy} holds for the HMC dynamics. Substituting the above expression of $h(a^l)$ to Eq.\eqref{eq:generic_entropy}, we have 
\begin{align*}
\log q^{L}(a^L)
%= & \log q^0(a^0) - \sum_{l = 0}^{L-1} \Tr \left( \nabla_{a^l} (v^l + (\epsilon/2)\nabla_{a^l} Q(s,a^l)) \right)\\
%\Tr \big((\epsilon^2/2) \nabla_{a^l}^2 Q(s,a^{l})\big) \\
= \log q^0(a^0) - \sum_{l = 0}^{L-1} (\epsilon^2/2) \Tr \big(\nabla_{a^l}^2 Q(s,a^{l})\big) 
\end{align*}
Unfortunately, this involves the computation of the Hessian of $Q(s,a^l)$, which is computationally more costly than that of SVGD-based sampler. Thus we choose to use the latter as the underlying sampler for our action sampling component.
\end{proof}

%\hp{Will put the first order derivative Lipschitz continuity condition in Theorem~\ref{thm:hmc_entropy}. Similarly, we can make assumptions of such to make sure $I + (\epsilon^2/2) \nabla_{a^l}^2 Q(s,a^t)$ is invertible (positive definite). This is useful: https://math.stackexchange.com/questions/1742753/lipschitz-implies-bounded-gradient}
% \begin{align*}
% \log q^{T}(a^T) &= \log q^0(a^0) - \sum_{t = 0}^{L-1} \log \Big| \det \nabla_{a^{l}} a^{l+1}  \Big| \\
%                 &= \log q^0(a^0) - \sum_{t = 0}^{L-1} \log \Big| \det \big(I +(\epsilon^2/2) \nabla_{a^l}^2 Q(s,a^{t-1})\big) \Big|
% \end{align*}
% According Jacobi's formula, given an invertible matrix $A$,
% \begin{align*}
% \log (\det A) = \Tr(\log A) \approx \Tr(A-I)
% \end{align*}
% Here the approximation holds when $\|A-I\|_{\infty}\ll 1$.

% Let $A=I + (\epsilon^2/2) \nabla_{a^l}^2 Q(s,a^t)$, then $\|A-I\|=(\epsilon^2/2) \nabla_{a^l}^2 Q(s,a^t)$, the above condition holds as long as the first order derivative $\nabla_{a^l} Q(s,a^t)$ is Lipschitz continuous along each dimension with a Lipschitz constant $L\ll 2/\epsilon^2$

% Hence, we have
% \begin{align*}
% \log q^{T}(a^T) = \log q^0(a^0) - \sum_{t = 1}^{T} \Tr \big((\epsilon^2/2) \nabla_{a^l}^2 Q(s,a^{t-1})\big) 
% \end{align*}
