# Supplementary material for: S$^2$AC: Energy-Based Reinforcement Learning with Stein Soft Actor Critic
Source: arXiv:2405.00987 source file (2024-05-02)
Supplement: Supplementary file 2 [file appendix_related_work_extension.tex]

\section{Related Work}

\subsection{Multi-modal Distribution Approximation}
\sanjay{Not sure if we need to have a discussion about MCMC/VI} \\
\xlp{Maybe we reduce content about MCMC,VI etc? For this section, we focus on high-level discussion about : multi-model distribution approximation}

To approximate intractable probability densities, Markov chain Monte Carlo (MCMC) sampling and variational inference (VI) are two popular methods. They are different approaches for solving same problem:  MCMC algorithms sample a Markov chain; variational algorithms solve an optimization problem. MCMC algorithms approximate the posterior with samples from the chain; variational algorithms approximate the posterior with the result of the optimization. Moreover, variational inference fits for large datasets while MCMC prefers smaller datasets and fits scenarios with a heavier computational cost for more precise samples. Furthermore, for approximating multimodal distribution, variational inference may perform better than general MCMC technique, even for small datasets.

\textbf{Markov chain Monte Carlo (MCMC):} MCMC algorithms are popular in statistics for solving all kinds of problems to obtain a sample from a complicated probability distribution. They are especially
useful for the purposes of Bayesian inference by allowing to sample from posterior distributions. Despite their popularity, MCMC techniques have their drawbacks. For example, the classical
MCMC methods, such as the Metropolis-Hastings algorithm or Hybrid Monte Carlo ~\citep{Duane}
are known to mix slowly between the modes if the target distribution is multimodal. Simiarly, Gibbs sampling is a powerful approach  to sampling from target distributions with multiple modes; but it quickly focuses on one of the modes ~\citep{David}.  There exists some enhanced versions, for example: adaptive MCMC for Multimodal Distributions ~\citep{Holmes2017AdaptiveMF} is proposed by introducing an auxiliary variable representing each mode and defining  an updated target distribution on an augmented state space. This adaptive scheme facilitates both local and jump moves.  Wormhole Hamiltonian Monte Carlo ~\citep{Lan2014WormholeHM} is another improved MCMC algorithm for sampling from multimodal
distributions, especially when the dimension is high and the modes are isolated.

\textbf{Varational Inference:}
In the varational inference derivations for approximating target distribution, the variational lower bound, also called evidence lower bound (ELBO), is an essential part. Since it is only a lower bound on the marginal log-likelihood of of observations, due to its simplicity,  one of the most commonly used variational distributions for the approximate posterior distribution of latent variable given by observation ($q(z|x)$) is the diagonal-covariance Gaussian. However, with such a simple variational distribution, the approximate posterior will most likely not match the complexity of the true posterior. An approach to achieve  flexible and complex distributions to match true posterior is to utilize normalizing flows. The main idea behind normalizing flow is to transform a simple (e.g., mean field) approximate posterior ($q(z|x)$) into a more expressive distribution by a series of successive invertible transformations.

\textbf{Score-based models:}
Recently, another way to represent probability distributions is to model the gradient of the log probability density function, a quantity often known as the (Stein) score function ~\citep{Liu}. Such score-based models are not required to have a tractable normalizing constant, and can be directly learned by score matching ~\citep{Hyvarinen}~\citep{Vincent}. Score-based models have achieved state-of-the-art performance on many downstream tasks and applications.

\sanjay{In model-free RL maximizing the combination of cumulative
reward and entropy has emerged as a key insight that encourages
efficient exploration and ultimately leads to a high-reward generating and stable policy. A challenge is how to estimate the entropy - especially in
non-parametric settings where we only have access to samples from a 
neural policy $\pi(a|s,\theta)$, but not its parametric form.}

\noindent
{\bf Entropy Estimation Variational Inference:} The Evidence Lower Bound (ELBO)

$\ln p_{\theta}(x) \geq \mathbb{E}_{q_{\phi}(z)}\left[\frac{ln p(x,z)}{q_{\phi}(z)}\right]$

\subsection{Entropy Estimator}
Entropy is a fundamental quantity in information theory and estimating entropy is important in the areas of computer science, machine learning, and data analysis. 
 
In most real-world applications, the underlying true probability density function (pdf) is rarely known, but samples from it can be obtained via
data-acquisition, experiments, or numerical simulations. The problem becomes to estimate the entropy of the underlying distribution only from a finite number of samples. The approaches are broadly be classified into two categories: parametric and non-parametric. 

(1) In the parametric approach the form of the pdf is assumed to be known and its parameters are identified from the samples. This, however, is a strong assumption and in most realistic cases an a priori assumption on the form of the pdf is not justified.

(2) For non-parametric approaches, there is no such assumption. One approach is to first estimate the pdf through histograms or kernel density estimators (KDE), and then to compute the entropy by either numerical or Monte-Carlo (MC) integration. Other alternatives include methods based on sample spacings for one-dimensional distributions and k-nearest neighbors (kNN). The kNN approach, also called Kozachenko-Leonenko (KL) estimator (Kozachenko \& Leonenko, 1987), is a widely used nonparametric estimator for the entropy of multivariate continuous random variables, which is based on statistics of k-nearest neighbor (kNN) distances (i.e., the distance from a sample to its kth nearest neighbor amongst the samples, in some metric on the space).

(3) In the variational inference method, the variational distribution $q_\phi (z)$ parameterized by $\phi$ is proposed to be represented by neural sampler, like the generator of GANs. The neural sampler is efficient to draw samples, but the entropy $H(q_\phi (z))$ is intractable since the density of $q_φ(x)$ is unknown. ~\citep{Taesup} and ~\citep{Zhai} propose several heuristics to approximate this entropy function. ~\citep{Kumar} propose to estimate the entropy through its connection to mutual information: H(qφ(z)) = I(gφ(z),z), which can be estimated from samples with variational lower bounds ~\citep{Nguyen}, ~\citep{Nowozin} and ~\citep{Belghazi}.
~\citep{Dai} notice that when defining
$p_{\theta}(x)= p_0(x)e^{−E_\theta(x)}/Z_\theta$, with $p_0(x)$ being a fixed base distribution, the entropy term $−H(q_\phi(x))$ equates $D_{KL}(q_\phi(x)|| p_0(x))$, which can be approximated with variational lower bounds using samples from $q_\phi(x)$ and $p_0(x)$, without requiring the density of $q_\phi(x)$.

\subsection{Exploration and Maximum-Entropy RL}
\textbf{Exploration in RL:}
Exploration is one of the most important issues in model-free RL, as there is the key assumption that all state-action pairs must be visited infinitely often to guarantee the convergence of Q-function. In order to explore diverse state-action pairs in the joint state-action space, various methods have been considered in prior works: intrinsically-motivated reward based on curiosity, model prediction error, information gain, and counting states . These exploration techniques improve exploration and performance in challenging sparse-reward environments. 

NOTE:  ~\citep{han2021max}

\textbf{Maximum Entropy RL:}
The maximum entropy framework has been considered in various RL domains: inverse reinforcement learning, stochastic optimal control, guided policy search, and off-policy learning . There is a connection between value-based and policy-based RL under the policy entropy regularization,  combines them, and finally proves that they are equivalent. Maximum entropy RL is also related to probabilistic inference. Recently, maximizing the entropy of state distribution instead of the policy distribution  and maximizing the entropy considering the previous sample action distribution have been investigated for better exploration. 

NOTE:  ~\citep{Han2021AME}

Maximum-Entropy RL augments the expected reward objective with an entropy maximization term. It optimizes policies to maximize both the expected return
and the expected entropy of the policy to achieve an improvement in exploration and robustness.

\textbf{Soft Q-learning (SQL):} SQL is a deep reinforcement learning framework for training maximum entropy policies in continuous state and action space ~\citep{Haarnoja_sql}. 
% The optimal policy has an energy-based form, and thus sampling from it becomes intractable in continuous and large action spaces. 
It learns a general conditional action distribution on a state: $\pi(a|s) \propto \exp(Q_\textit{soft}(s,a))$ and uses approximate inference based on amortized Stochastic Variational Gradient Descent (SVGD)~\citep{liu2016stein,wang2016learning} to optimize ``particles'' to approximate the distribution, resulting in multimodal exploration and policies that can be more easily adapted to new environments. 

A key advantage of SVGD is that it proves the equivalence between the derivative of the KL-divergence and the Stein-operatior, thus derives a closed-form solution of the derivative of the KL-divergence.} 

However, SQL uses a deep sampling network to both draw samples from $\pi(a|s)$ as well as act as a stochastic (non-deterministic) actor. Experiments on mujoco tasks show soft Q-learning can learn all tasks, but it is slower than SAC and has worse asymptotic performance. Zhang et. al.~\cite{rzhang_wass} reinterpret SQL with gradient flows in a space of probability distributions metrized by Wasserstein
distance. However, this approach suffers from high computational cost as well as inaccuracy due to the sampling-based approximation of derivative of the Wasserstein distance.  

\textbf{Soft Actor Critic (SAC):} SAC ~\citep{Haarnoja_sac} is an off-policy actor-critic which  has a stochastic actor (contrary to DDPG)  being more optimal and sample efficient than on-policy methods such as A3C or PPO. SAC builds on SQL to solve these issues and also avoids the complexity and potential instability associated with approximate inference 
based on soft Q-learning.

 SAC uses a Gaussian mixture model policy and a entropy regularized Q-function. A key feature of SAC, and a major difference with common RL algorithms, is that it is trained to maximize a trade-off between expected return and entropy, a measure of randomness in the policy. The aim is to train a maximum entropy which will naturally
encourage exploration. The target for Q-learning becomes $r + \gamma (1 - d)Q^{\theta_i}(s,a)) - \alpha*\log(\pi(a|s))$. 

However, the weaknesses of SAC are that it learns maximum entropy policies restricted to parameterized families of tractable policy distributions and it generates high-variance using automatic temperature tuning. SAC requires a parameterized distribution (for entropy optimization) which may be unknown in most practical applications. 

\textbf{Max-Min entropy RL:}
Furthermore, using sample-based update with function approximation, however, the SAC iteration does not yield the desired result, contrary to the intention behind maximum entropy.  ~\citep{han2021max} studied the limitation of maximum entropy SAC.  One experiment  on pure exploration task demonstrates that SAC fails to converge to the optimal uniform policy and its performance become saturated.  The authors propose a max-min entropy framework to overcome the limitation of the SAC algorithm  in model-free sample-based learning, which aims to learn policies reaching states with low entropy and maximizing the entropy of these low-entropy states, whereas the conventional maximum entropy RL optimizes for policies that aim to visit states with high entropy and maximize the entropy of those high-entropy states for high entropy of the entire trajectory. 
The approach learns the Q-function to estimate the negative sum of policy entropy, while maintaining the policy entropy maximization term $\mathcal{H}(\pi(\cdot|s_t))$ in the policy update to increase the policy entropy of the visited states.

\textbf{Meta-SAC for Temperature hyperparameter:}
SAC (Haarnoja et al., 2018a) (referred to as SAC-v1 throughout) is known to be particularly sensitive to the entropy temperature. For large temperature, the policy is encouraged to become nearly uniform and thus fails to exploit the reward signal, which substantially degrading the performance; for small temperature, though the policy learns quickly at first, it then becomes nearly deterministic and gets stuck at poor local minimal due to lack of exploration. However, it is non-trivial to choose a proper value of the entropy temperature. The optimal value not only changes across different tasks, but also varies in the learning process as the policy improves. In SAC-v1, this problem is solved by treating α as a hyperparameter and determining its value by grid search. This brings significant computational costs and manual efforts, and needs to be done for each new task.  In the follow-up work (SAC-v2), which uses constrained optimization for automatic adjustment by introducing another hyperparameter
“target entropy”, which by itself needs to be tuned for each task. The authors give a heuristic formula for choosing this new hyperparameter, which performs empirically well on Mujoco tasks, however, it remains unknown whether it is the optimal choice for every task. Meta-SAC ~\citep{Yufei} propose to leverage the metagradient method (Xu et al., 2018; Zheng et al., 2018) and a novel meta loss to automatically tune the value of α during the learning process without having  any adaptive hyperparameters. Experiment results show that Meta-SAC can be a strong alternative to SAC-v2, especially for complex tasks. 

NOTE: ~\cite{Yufei}

\textbf{Robustness of MaxEnt RLs:} Many real-world applications of reinforcement learning (RL) require guarantees that the agent will perform well in the face of disturbances to the dynamics or reward function. ~\citep {Eysenbach2022MaximumER} prove theoretically that maximum entropy (MaxEnt) RL, including SAC, maximizes a lower bound on a robust RL objective, and thus can be used to learn policies that are robust to some disturbances in the dynamics and the reward function. However, MaxEnt RL methods are not necessarily the ideal approach to robustness: applying such methods still requires choosing a hyperparameter (the entropy coefficient), and the robust set for MaxEnt RL is not always simple. 

NOTE: ~\cite{Eysenbach2022MaximumER}

\textbf{Multimodality:}
A multimodal policy search aims to learn a policy that can capture the multimodality of optimal actions. Many previous policy search-based methods employ a hierarchical policy model that consists of low-level policies that determine robot action and a high-level policy that determines which low-level policy is used [25, 26, 27, 28]. However, the proposed approaches employ such hierarchical parametric models as 1) a softmax gating function with linear Gaussian sub-policies or 2) Gaussian mixture models with a parametric policy model, both of which require hand-engineered features to cope with high-dimensional sensor input, unlike non-parametric methods.
Multimodality in optimal action has also been considered in neural network- based RL methods. For example, soft Q-learning learns a value function to acquire diverse behaviors by introducing an entropy term in the Bellman equation that promotes capturing multimodality in policies [29]. Soft actor-critic (SAC) is an extension of soft Q-learning; the learning performance is greatly improved [30, 31]. In the SAC algorithm, although the value function captured multiple optimal,  the policy employs a unimodal model. Thus, it cannot explicitly capture multi- modality in optimal actions. SAC-GMM with a GMM policy was also explored as an early version of SAC, but its performance is worse than SAC due to the algorithmic complexity [32]. Kalashnikov et al. proposed another method that selects an action from an action-value function using the cross-entropy method [33].  ~\citep{Sasaki2021VariationalPS}  propose a multimodal SGP-PS that employs a policy model inspired by the overlapping mixtures of Gaussian processes (OMGP). Multimodal SGP-PS learns a policy whose components in the mixture are global and overlapping in state space. In table-sweeping task experiments, the multimodal SGP policy learned the multiple optimal actions for sweeping an object in each initial state by the nature of multimodality. 

NOTE: ~\citep {Sasaki2021VariationalPS}

\textbf{Diffusion RLs:}

(1) Diffuser:  Diffuser ~\citep{Janner} applies a diffusion model as a trajectory generator. The full trajectory of state-action pairs are grouped together to form a single sample for the diffusion model. A separate return model is learned to predict the cumulative rewards of each trajectory sample. The guidance of the return model is then injected into the reverse sampling stage. This approach is similar to Decision Transformer ~\citep{Chen}, which also learns a trajectory generator through GPT2 ~\citep{Radford} with the help of the true trajectory returns. When used online, sequence models can no longer predict actions from states autoregressively (since the states are an outcome of the environment). Thus, in the evaluation stage, a whole trajectory is predicted for each state while only the first action is applied, which incurs a large computational cost.

(2)Diffusion-QL:
Recently, Diffusion-QL ~\citep{Zhendong}, a new offline RL algorithm, leverages conditional diffusion model as a highly expressive policy class for behavior cloning and precise policy regularization to learn optimal actions.  From various experiments, it shows Diffusion-QL outperforms most of the prior methods on the D4RL benchmark tasks.  

 Diffusion-QL has many nice properties: (1) diffusion models are very expressive and can well capture multi-modal distributions. (2) the diffusion model loss constitutes a strong distribution matching technique even in the image generation case, and hence it could be seen as a powerful sample-based policy regularization method without the need for extra behavior cloning. (3) diffusion models perform generation via iterative refinement, and the guidance from maximizing the Q-value function can be added at each reverse diffusion step.

 The objective of constructing diffusion loss is composed 1) a behavior-cloning term that encourages the diffusion model to sample actions in the same distribution as the training set, and 2) a policy improvement term that attempts to sample high-value actions (according to a learned Q-value). Diffusion-QL builds a multilayer perceptron (MLP) based denoising diffusion probabilistic model (DDPM) ~\citep{Ho} as model policy, which is a conditional model with states as the condition and actions as the outputs. 

While both Diffuser ~\citep{Janner} and  Diffusion-QL apply diffusion models in Offline RL, Diffuser is from the trajectory-planning perspective while  Diffusion-QL is from the offline policy-optimization perspective.

NOTE: ~\citep{Zhendong}

\subsection{Stein Variational Gradient Descent}
SVGD starts with a initial set of random particles and sequentially
applies functional gradient descent to minimize the KL-divergence
between the current and the target distribution. The functional
gradient is taken in the space of probability distributions equipped
with Wasserstein metric

SVGD update rule:
\[
a^{l+1}_{i} \leftarrow a^{l}_{i} + \epsilon\underbrace{\frac{1}{m}\sum_{j=1}^{m}\left[k(a^{l}_{i},a^{l}_{j})\nabla_{a^{l}_j}Q(s,a^{l}_{j}) + \nabla_{a^{l}_{j}}k(a^{l}_i,a^{l}_j)\right]}_{\text{$Q(a^{l}_i, s)$}}
\]

produce unbiased samples from the energy based model using amortized Stein variational gradient descent to learn a stochastic sampling network that approximates samples from this distribution.

\section{Our Approach}
We model the policy as an exponential distribution over Q-values $\pi(a_t|s_t) \propto \exp{Q(s_0,\cdot)}$.

\begin{eqnarray*}
\pi^{*}(\cdot|s_t)&=&\argmin_{\pi} D_{KL}(\pi(\cdot|s_0) \| \frac{\exp{Q(s_0,\cdot)}}{Z} ) \\
&=& \argmax_{\pi}\mathbb{E}_{\pi}  \Big[ Q(s_0,a_0) - \log \pi(a_0|s_0)   \Big] \\
&=& \argmax_{\pi}\mathbb{E}_{\pi}  \Big[ \sum_t r(s_t,a_t) + \mathcal{H}(\pi(\cdot|s_t))  \Big]
\end{eqnarray*}

\noindent$\mathcal{H}(\pi(\cdot|s_t))$ is the entropy of the actions distribution at a state $s_t$. 

\noindent This adds robustness: entropy is like injecting noise during training 
\\

\noindent\textit{Soft Actor Critic (SAC)}:\\
%learns $Q^{\pi}$ and $\pi$ jointly. It's much more stable and scalable in practice. 
\noindent \textit{Step1}: Update Q-function to evaluate the current policy:

\begin{equation*}
Q(s,a) \leftarrow r(s,a) + \mathbb{E}_{s' \sim p_s ,a'\sim \pi}  \Big[ Q(s',a') - \log \pi(a'|s')  \Big]
\end{equation*}

\noindent \textit{Step2:} Update the policy

\begin{equation*}
\pi = \argmin_{\pi} D_{KL} ( \pi(\cdot |s ) \|\frac{ \exp{Q(s,\cdot)}}{Z}  )
\end{equation*}
 
\noindent In practice: $\pi$ is modeled as a Gaussian distribution \\

\noindent Limitation of SAC: no multi-modality, quickly commits to one mode during training. What happens in practice is that it explores the surroundings of one mode instead of exploring several modes.

\noindent {\color{blue} Validating experiment: In multi-modal Gaussian environment, the standard deviation of the policy drops quickly and stays constant across states. SAC coomits quickly to one mode and fails at capturing multi-modality as a result. }\\

\noindent We propose STAC which models the policy as a multi-modal distribution to improve exploration around local optimum.\\

\begin{comment}

\textit{Soft Q-learning (SQL)}: Learns $Q^{*}$ directly then sample $a^{*}_{t}$ for $\pi^{*}(a_t|s_t) \propto \exp{Q^{*}(s_t,a_t)}$. Sampling is however intractable for continuous actions. Instead, use approximate inference procedure to sample (Stein variational gradient descent).\\

Related work: Soft Q-learning (SQL) Haarnoja & tang et al 2017
Soft Actor Critic (SAC) Haarnoja & al 2018
Path Consistency Learning (PCL) Nachum et al 17
other related algorithms: Todorov 07, Ziebart 08, Toussain 09, Rawlik et al 12, Fox et al 16  
\end{comment}

\paragraph{Connections to maximum entropy RL/IRL approaches and guided policy search} This would include SQL and SAC. Inverse RL~\cite{ziebart2008maximum}, SVPG~\cite{liu2017stein}. Also this one~\cite{fujimoto2019off} on batch RL that combines the views from imitation learning and off-policy RL. Here VAE is used instead of GAN. The related work from SAC provides a nice discussion that we could start with.

\hp{In some sense, guided policy search is like imitation learning, where the policy that we want to learn is either to be restricted to be close to some target policy (in guided policy search, trust region methods, and energy based methods), or to directly mimic the behavior policy (in imitation learning). Papers connecting GANs and inverse RL/imitation learning~\cite{finn2016connection,ho2016generative}.}
