# Supplementary material for: S$^2$AC: Energy-Based Reinforcement Learning with Stein Soft Actor Critic
Source: arXiv:2405.00987 source file (2024-05-02)
Supplement: Supplementary file 3 [file proof_ld_likelihood.tex]

\textbf{Closed for expression of Langevin dynamics Induced Policy}
Langevin dynamic update rule: $a^{l+1}_{i} \leftarrow a^{l}_{i} + \epsilon, g(a^{l}_{i})$, with 

\begin{equation}
g(a^{l}) = \epsilon \nabla_{a^{l}} Q(a^{l},s) + \eta 
\end{equation}

We follow a similar procedure as above and obtain:

\begin{eqnarray*}
\log p(a^{L}|s)&=&\log p(a^{0}|s)-\sum_{l=0}^{L-1}\log \Big|\det \frac{a^{l+1}}{a^{l}} \Big|\\
&=&\log p(a^{0}|s)-\sum_{l=1}^{L-1}\log \Big|\det \Big(I + \epsilon \nabla_{a^{l}} g(a^{l})\Big) \Big|\\
&\approx& \log p(a^{0}|s)-\sum_{l=0}^{L-1}\epsilon \, \text{tr} \Big(\nabla_{a^{l}} g(a^{l})\Big)\\
&=& \log p(a^{0}|s)-\sum_{l=0}^{L-1} \epsilon^{2} \text{tr} \left( \nabla_{a^{l}}^{2} Q(a^{l},s)\right) \\
\end{eqnarray*}

In case the Hessian is symmetric, we can actually compute the trace with just vector operations.

It's possible to compute a stochastic estimator of the trace using the Hutchinson trick: $tr(A)= \mathbb{E}_{z}[z^T A z]$. with $z$ being random variables satisfying $\mathbb{E}_{z}[zz^T]=I$, for instance $z$ can be radamacher randomvariables or be drawn from a normal distribution. 

\begin{equation}
\text{tr}(\nabla_{a^{l}}^{2} Q(a^{l},s)) = \mathbb{E}_{z}[z^T \nabla_{a^{l}}^{2} Q(a^{l},s)  z]= \mathbb{E}_{z}[z^T \nabla_{a^{l}}\left(\nabla_{a^{l}} Q(a^{l},s)^T  z \right)]
\end{equation}
